# Supplementary material for: Diffuse Adiabatic Flows in Thermally Coupled Grounded Shallow Ice Sheets: Modelling and Analysis
Source: arXiv:2606.14258 source file (2026-06-29)
Supplement: Supplementary file 1 [file appendix.tex]

\section{title}\label{app:A}

hello
